# Supplementary material for: Two-Layer Attention Optimization for Bimanual Coordination
Source: arXiv:2411.07470 source file (2025-03-14)
Supplement: Supplementary file 1 [file appendix.tex]

\appendix
